# Supplementary material for: Statistical hydraulic model for the Leonardo's rule
Source: arXiv:2009.10310 ancillary file (2020-09-22)
Supplement: Supplementary file 1 [file Suppl-Info-Leonardos-rule.pdf]

# Supplementary Information for "Statistical hydraulic model for the Leonardo's rule"

by O. Sotolongo-Costa et al*

## I. TECHNICAL SHEETS OF TREES

*Quercus rugosa*

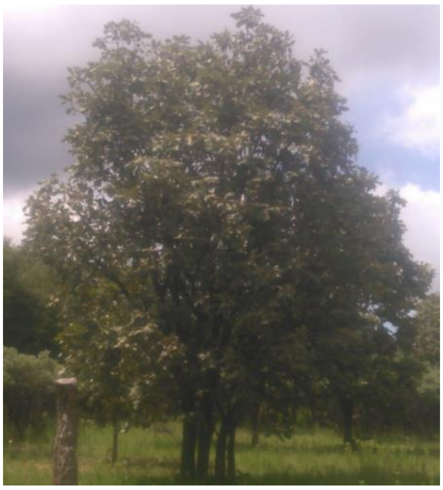

FIG. 1. *Quercus rugosa.*

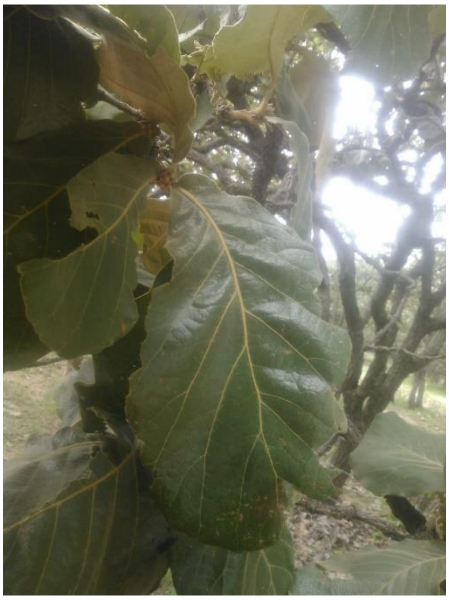

FIG. 2. *Quercus rugosa*

**Scientific name:** *Quercus rugosa.*

**Common Name:** White oak.

**Family:** Fagaceae.

**Nativity:** North America.

**Location:** Palo Herrado in Nochistlán de Mejía; Zacatecas.

**Aerial part:** Wide and rounded crown that provides dense shade.

**Height:** Tree up to 30 m tall (depending on available moisture).

**Trunk diameter:** Tree up to 1 m wide.

**Climate:** Temperate and semi-cold climates.

**Soil:** Prefers moist soils.

**Root system:** Deep.

**Duration:** Perennial.

**Leaves:** Unlobed, obovate, oblanceolate, or elliptic, 2-10 cm long, 1.5-7 cm wide.

**Flowers:** Wind pollinated staminate aments, with reduced perianth parts, 3-6 stamens.

**Fruit:** Acorns 1.5-2 cm long, usually 2-4 on peduncles 1.5-6.3 cm long, finely appressed yellowish or reddish pubescent to woolly within; scales with thickened bases.

**Propagation**: Seed.

*Eucalyptus camaldulensis*

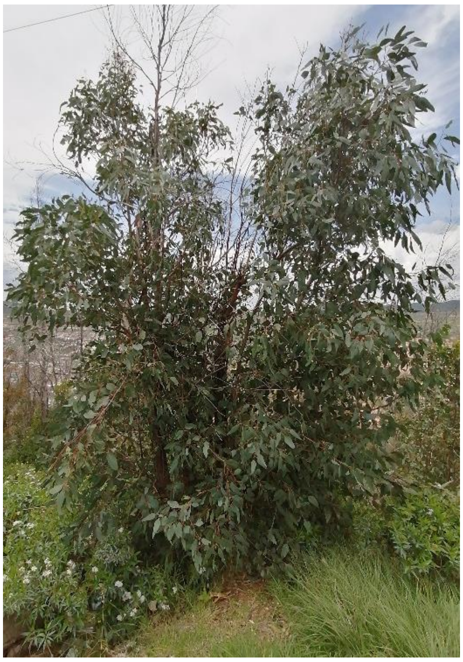

FIG. 3. *Eucalyptus camaldulensis*

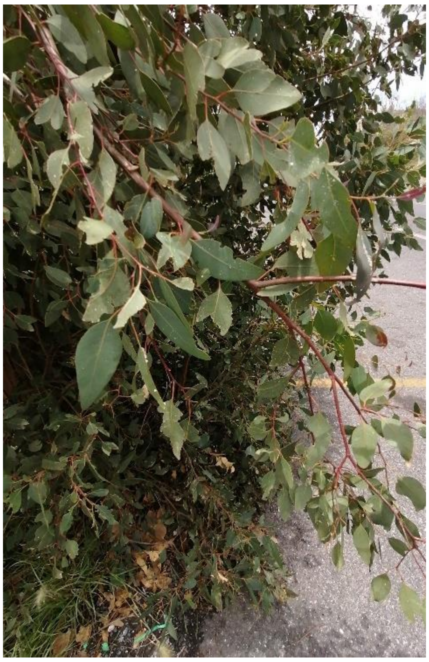

FIG. 4. *Eucalyptus camaldulensis*

**Scientific name:** *Eucalyptus camaldulensis.*

**Common Name:** Red Gum, River Red Gum, Eucalyptus.

**Family:** Myrtaceae.

**Origin:** Australia.

**Location:** Cerro de la Bufa in Zacatecas; Zacatecas.

**Aerial part:** Evergreen, highly branched, with a small crown.

**Height:** Tree up to 50 m tall.

**Trunk diameter:** Tree up to 2 m wide.

**Climate:** Grows in arid and semi-arid areas.

**Soil:** Acidic or Sandy alluvial soils and colonizes natural areas with moisture.

**Root system:** Extensive and deep.

**Duration:** Perennial.

**Leaves:** The leaf is slightly ovate to oblong, green to gray-green.

**Flowers:** The white flowers bloom in groups of five to ten mainly in the late spring and summer and followed by small light brown seed capsules. Flowers up to 1 cm in diameter.

**Fruit:** Fruit hemispherical, to 0.6 mm long and 1 cm wide, on a very short stalk, the valves exserted. Flowering summer.

**Propagation**: Seed.

*Schinus molle*

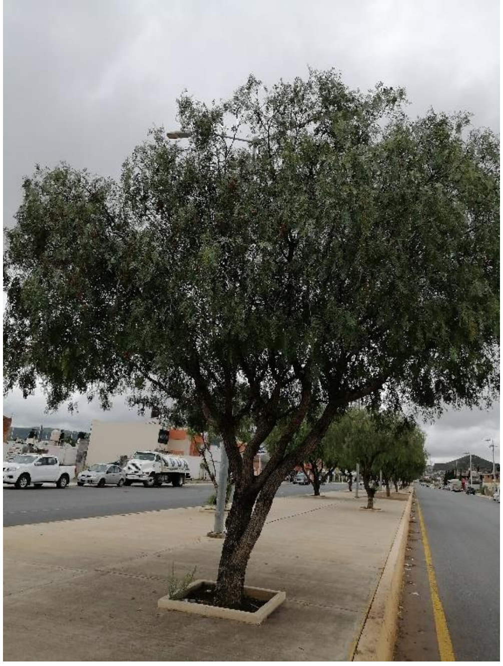

FIG. 5. *Schinus molle*

**Scientific name:** *Schinus molle.*

**Common Name:** Peruvian Peppertree, Pirul.

**Family:** Anacardiaceae.

**Origin:** South America.

**Location:** Av. Siglo XXI in Guadalupe; Zacatecas.

**Aerial part:** Round and elegant crown.

**Height:** Tree up to 17 m tall.

**Trunk diameter:** Tree up to 1.5 m wide.

**Climate:** Temperate, it does not tolerate low temperatures for a long time.

**Soil:** Sandy and clay.

**Root system:** Extensive and shallow.

**Duration:** Perennial.

**Leaves:** Pinnately compound leaves measure 8–25 cm long, 4–9 cm wide and are made up of 19-41 alternate leaflets.

**Flowers:** Flowers are small, white and borne profusely in panicles at the ends of the drooping branches, they measure 6 mm crosswise.

**Fruit:** The fruit are 5–7 mm diameter round drupes with woody seeds that turn from green to red, pink or purplish.

**Propagation**: Seed.

*Prunus serotina*

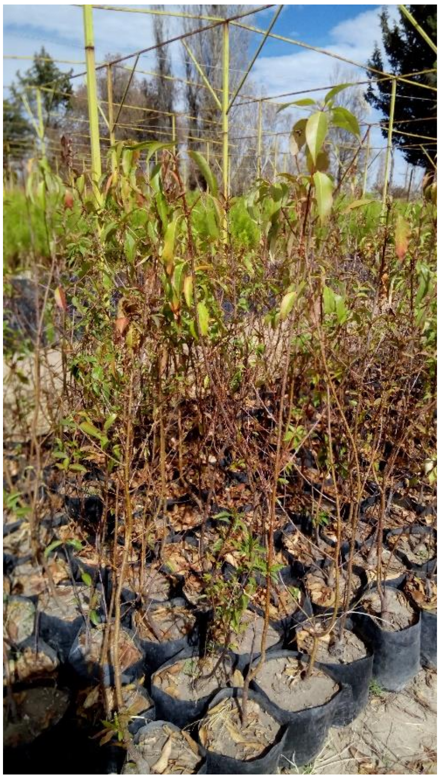

FIG. 6. *Prunus serotina*

**Scientific name:** *Prunus serotina.*

**Common Name:** Black Cherry, Capulín.

**Family:** Rosaceae.

**Nativity:** North America.

**Location:** General de Enrique Estrada; Zacatecas. Vivero de Comisión Nacional Forestal (CONAFOR) of Zacatecas.

**Aerial part:** Wide ovoid-shaped crown that produces a dense shade.

**Height:** Tree up to 10 m – 15 m tal.

**Trunk diameter:** Tree up to 1.2 m wide.

**Climate:** Temperate and cold.

**Soil:** Stony dark, shallow, deep with abundant organic material.

**Root system:** Widely extended.

**Duration:** Perennial.

**Leaves:** Alternate, simple, oblong-ovate to lance-ovate, 5-12 cm long and 2.5-4.5 cm wide, tip acuminate.

**Flowers:** Flowers white, 8 mm wide, in 12 cm long clusters (racemes).

**Fruit:** Fruit 9 mm diameter., round, turns black in early fall.

**Propagation:** Seed.

## II. IMAGE PROCESSING METHODS

With the first image processing method the radius of xylem structures like tracheids and vessel elements is measured directly with the tools of ImageJ software. In specific, the ImageJ tools allow us to obtain the diameter of the xylem structures by drawing a transverse line as shown in Fig. 7a. The diameter is obtained in pixels and then transformed to microns.

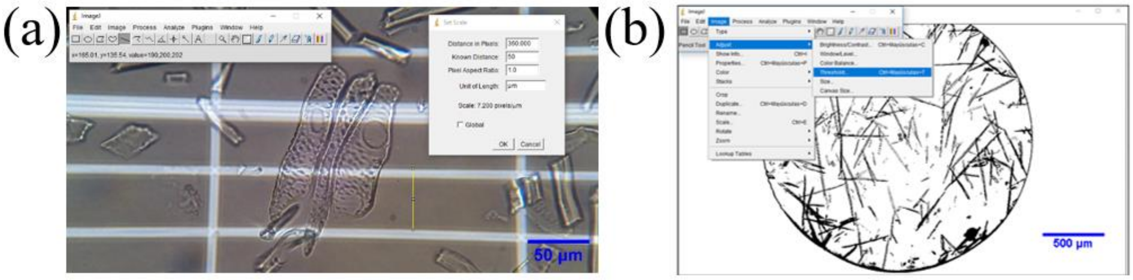


FIG. 7. Image processing methods for the determination of the size distribution of the xylem elements. (a) The diameter (radius) of the xylem structures is directly measured with the ImageJ line tool. (a) The area of conducting and non-conducting elements is measured automatically once the sample images are black and white contrasted. The radius of the xylem elements is indirectly obtained by assuming the golden mean for the proportion between the length and the width of a xylem element.

With the second image processing method, we obtain the size distribution of the xylem elements by measuring automatically the area of all conducting structures once the sample images have been black and white contrasted, see Fig. 7b. To determine the radius (width) of the xylem elements we assume that the relationship between length and width is such that the golden mean is valid. In Fig. 8 we show the mentioned proportion between the width and length of a xylem element.

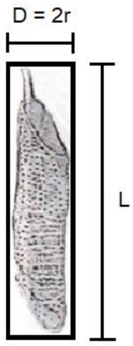


FIG. 8. Proportion between the length and width of a xylem element. We assume that the proportion obeys the golden mean $\phi = L/D \approx 1.61$, being the same for all xylem elements. By measuring the area of a xylem element we can obtain its radius as $r = \sqrt{\frac{A}{4\phi}}$.

The area of a xylem element is given as

$$A = LD, \tag{1}$$

where $L$ and $D$ are the length and width of a xylem element. The golden mean

$$\phi = \frac{L}{D} = \frac{1 + \sqrt{5}}{2} \approx 1.61, \tag{2}$$

allows us to relate straightforwardly the area and diam- eter (width) by replacing the length of Eq. (1) in Eq. (2)

$$\phi = \frac{A}{D^2}, \tag{3}$$

or equivalently in terms of the radius (D = 2r)

$$r = \sqrt{\frac{A}{4\phi}} \approx \sqrt{\frac{A}{6.47}} \tag{6}$$
